# Supplementary material for: Separating deterministic and stochastic gravitational wave signals in realistic pulsar timing array datasets
Source: arXiv:2407.21105 source file (2024-07-30)
Supplement: Supplementary file 1 [file appendix_a.tex]

\section{S/N}

\begin{figure}[ht]
    \centering
    \includegraphics[width=0.5\textwidth]{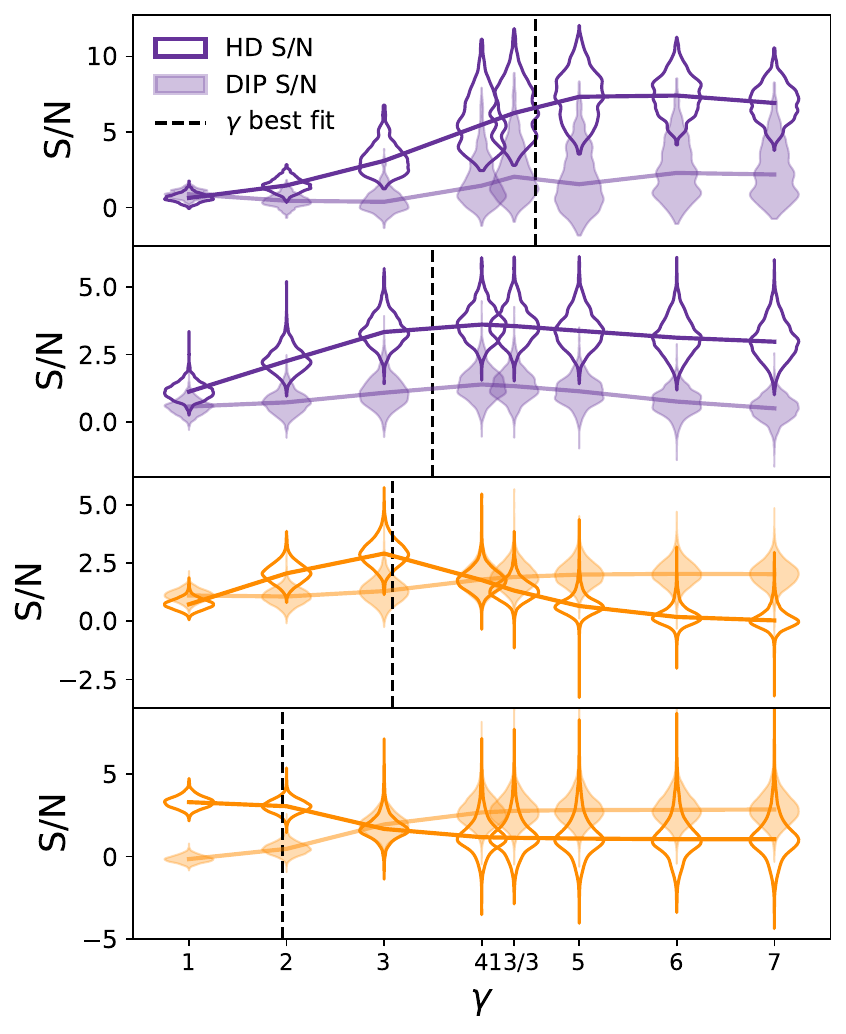}
    \caption{}
    \label{fig:HDDIP_SNR}
\end{figure}
